# Supplementary material for: Wakening Past Concepts without Past Data: Class-Incremental Learning from Online Placebos
Source: arXiv:2310.16115 source file (2023-10-24)
Supplement: Supplementary file 1 [file ablation_1_appendix.tex]

\setlength{\tabcolsep}{1.9mm}{
\begin{table*}[ht]
  \small
  \centering
  %\vspace{-0.3cm}
  \begin{tabular}{llccccccccccccc}
  \toprule
    \multirow{2.5}{*}{Method} & \multicolumn{2}{c}{20 exemplars/class} && \multicolumn{2}{c}{10 exemplars/class} && \multicolumn{2}{c}{5 exemplars/class}\\
  \cmidrule{2-3} \cmidrule{5-6} \cmidrule{8-9}
    & Average & Last  && Average & Last && Average & Last \\
    \midrule

    iCaRL & 48.22 \tiny{\whitet{+1.35}} & 39.56 \tiny{\whitet{+3.64}} && 40.40  \tiny{\whitet{+3.64}} & 33.14 \tiny{\whitet{+3.64}} && 32.53  \tiny{\whitet{+13.64}} & 19.35 \tiny{\whitet{+13.64}}\\
    \cellcolor{mygray-bg}{\ \ \emph{w/} ours} &  \cellcolor{mygray-bg}{52.46 \tiny{\redt{+4.24}}} & \cellcolor{mygray-bg}{42.01 \tiny{\redt{+2.45}}} & \cellcolor{mygray-bg}{} & \cellcolor{mygray-bg}{42.48 \tiny{\redt{+2.08}}} & \cellcolor{mygray-bg}{33.20 \tiny{\redt{+0.06}}} & \cellcolor{mygray-bg}{} & \cellcolor{mygray-bg}{36.40 \tiny{\redt{+3.87}\grayt{1}}} & \cellcolor{mygray-bg}{22.70 \tiny{\redt{+3.35}\grayt{1}}}\\
     \\[-12pt]
\cmidrule{1-9}

    LUCIR & 57.54 \tiny{\whitet{+1.35}} & 48.32 \tiny{\whitet{+3.64}} && 49.78  \tiny{\whitet{+13.64}} & 40.63 \tiny{\whitet{+13.64}} && 45.64 \tiny{\whitet{+13.64}} & 32.16 \tiny{\whitet{+13.64}}\\
   \cellcolor{mygray-bg}{\ \ \emph{w/} ours} &  \cellcolor{mygray-bg}{63.66 \tiny{\redt{+6.12}}} & \cellcolor{mygray-bg}{53.77 \tiny{\redt{+5.45}}} & \cellcolor{mygray-bg}{} & \cellcolor{mygray-bg}{61.22 \tiny{\redt{+11.44}}} & \cellcolor{mygray-bg}{50.84 \tiny{\redt{+10.21}}} & \cellcolor{mygray-bg}{} & \cellcolor{mygray-bg}{59.82 \tiny{\redt{+14.18}}} & \cellcolor{mygray-bg}{48.83 \tiny{\redt{+16.67}}}\\
    \\[-12pt]
    \cmidrule{1-9}
    
   LUCIR+AANets & 64.29 \tiny{\whitet{+1.35}} & 52.99 \tiny{\whitet{+3.64}} && 59.75  \tiny{\whitet{+3.64}} & 48.19 \tiny{\whitet{+3.64}} && 55.26  \tiny{\whitet{+13.64}} & 39.60  \tiny{\whitet{+12.28}}\\
    \cellcolor{mygray-bg}{\ \ \emph{w/} ours} &  \cellcolor{mygray-bg}{65.96 \tiny{\redt{+1.67}}} & \cellcolor{mygray-bg}{57.67 \tiny{\redt{+4.68}}} & \cellcolor{mygray-bg}{} & \cellcolor{mygray-bg}{63.60 \tiny{\redt{+3.85}}} & \cellcolor{mygray-bg}{52.67 \tiny{\redt{+4.48}}} & \cellcolor{mygray-bg}{} & \cellcolor{mygray-bg}{63.01 \tiny{\redt{+7.75}\grayt{1}}} & \cellcolor{mygray-bg}{51.88 \tiny{\redt{+12.28}}}\\
     \\[-12pt]
    \cmidrule{1-9}

    POD+AANets & 62.12  \tiny{\whitet{+1.35}} & 51.73 \tiny{\whitet{+3.64}} && 53.31  \tiny{\whitet{+3.64}} & 42.83 \tiny{\whitet{+3.64}} && 45.09  \tiny{\whitet{+13.64}} & 32.97  \tiny{\whitet{+13.64}}\\
      \cellcolor{mygray-bg}{\ \ \emph{w/} ours} &  \cellcolor{mygray-bg}{64.53 \tiny{\redt{+2.41}}} & \cellcolor{mygray-bg}{54.95 \tiny{\redt{+3.22}}} & \cellcolor{mygray-bg}{} & \cellcolor{mygray-bg}{58.75 \tiny{\redt{+5.44}}} & \cellcolor{mygray-bg}{46.83 \tiny{\redt{+4.00}}} & \cellcolor{mygray-bg}{} & \cellcolor{mygray-bg}{47.86 \tiny{\redt{+2.77}\grayt{1}}} & \cellcolor{mygray-bg}{33.93 \tiny{\redt{+0.96}\grayt{1}}}\\
       \\[-12pt]
    
  \bottomrule

\end{tabular}
  \caption{\suppt{Supplementary to Table~\ref{table_ablation_exemplars}.}
  Evaluation results (\%) on $25$-Phase CIFAR-100 using  POD+AANets~\citep{Liu2020AANets}, LUCIR+AANets~\citep{Liu2020AANets}, LUCIR~\citep{hou2019lucir}, and iCaRL~\citep{rebuffi2017icarl} \emph{w/} and \emph{w/o} our PlaceboCIL plugged in.
  ``Average'' and ``Last'' denote the average accuracy over five phases and the last-phase ($25$-th) accuracy, respectively.
}
% \vspace{-6mm}
  \label{table_ablation_exemplars_appendix}
\end{table*}
}
